# Supplementary material for: Regularizing Model Complexity and Label Structure for Multi-Label Text Classification
Source: arXiv:1705.00740 source file (2017-05-01)
Supplement: Supplementary file 1 [file appendix.tex]

%!TEX root = ./body.tex
